# Supplementary material for: Migration barriers for diffusion of As and P atoms in InP and InAs via vacancies and interstitial atoms
Source: arXiv:2404.01607 source file (2024-04-02)
Supplement: Supplementary file 1 [file Supplementary_material.pdf]

# Supplementary material to “Migration barriers for diffusion of As and P atoms in InP and InAs via vacancies and interstitial atoms”

Ivan A. Aleksandrov, Konstantin S. Zhuravlev

Rzhanov Institute of Semiconductor Physics, Siberian Branch of Russian Academy of Sciences,  
Novosibirsk, Russia

## 1. Defect formation energies in InP and InAs in the generalized gradient approximation

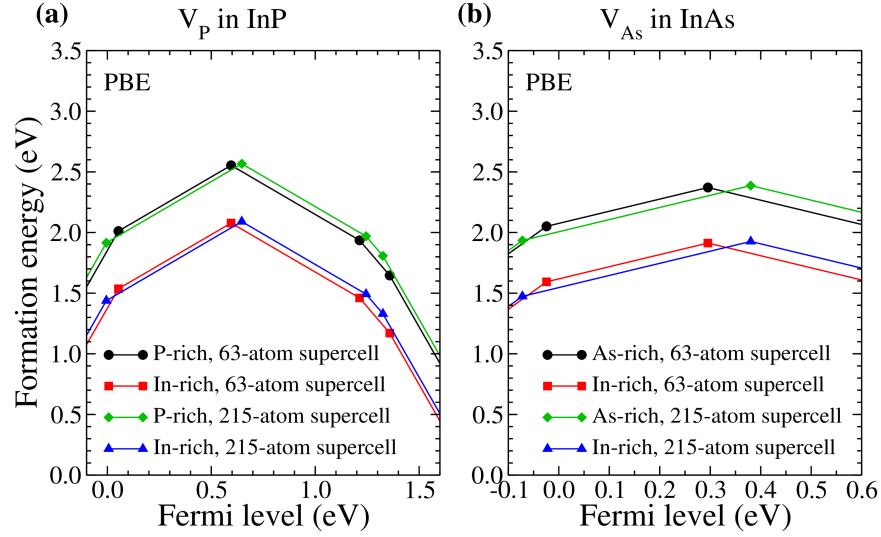

**Figure S1.** Dependence of the phosphorous vacancy formation energy in InP on the Fermi level for P-rich and In-rich conditions (a) and dependence of the arsenic vacancy formation energy in InAs on the Fermi level for As-rich and In-rich conditions (b). Calculation in the generalized gradient approximation with the PBE functional for the 63-atom and 215-atom supercells.

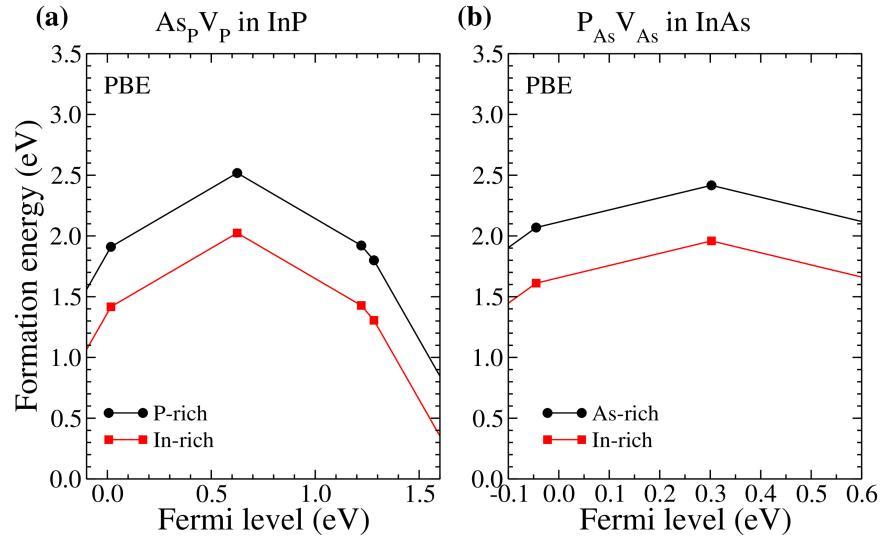

**Figure S2.** Dependence of the formation energies of the  $As_P V_P$  complex in InP (a) and  $P_{As} V_{As}$  complex in InAs (b) on the Fermi level. Calculation in the generalized gradient approximation with the PBE functional for the 63-atom supercell.

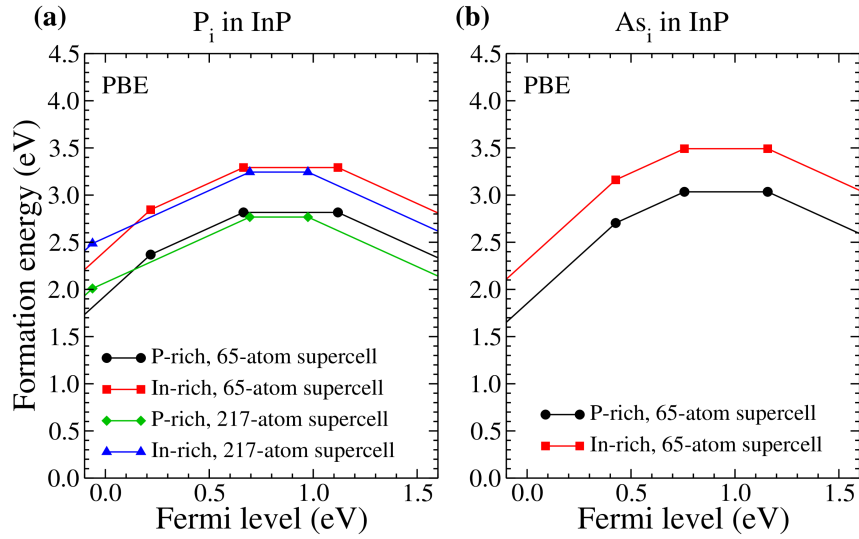

**Figure S3.** Dependence of the formation energy of interstitial phosphorous (a) and arsenic (b) atoms in InP on the Fermi level for P-rich and In-rich conditions. Calculation in the generalized gradient approximation with the PBE functional for the 65-atom and 217-atom supercells.

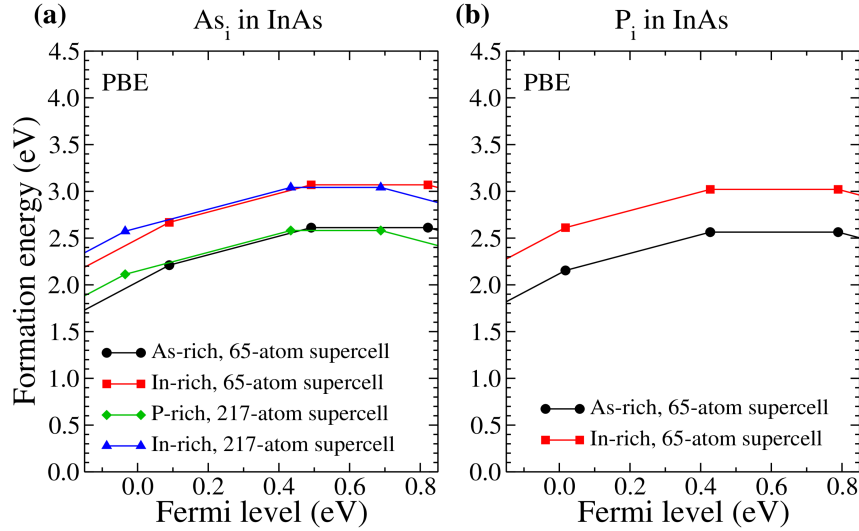

**Figure S4.** Dependence of the formation energy of the interstitial As atoms (a) and interstitial P atoms (b) in InAs on the Fermi level for As-rich and In-rich conditions. Calculation in the generalized gradient approximation with the PBE functional for the 65-atom and 217-atom supercells.

**Table S1.** Symmetry of  $V_P$  in InP and interatomic distances for indium atoms nearest to the vacancy in different charge states. Calculation with PBE functional for supercell sizes of 63 and 215 atoms. If the In-In interatomic distances are different, their number is given in parentheses for each distance. If several different configurations with close total energies are found, the difference in total energies  $\Delta E$  is shown for them relative to the configuration with the minimum energy in a given charge state.

| PBE, 63-atom supercell |          |                              |                 |
|------------------------|----------|------------------------------|-----------------|
| Charge                 | Symmetry | In-In distances, Å           | $\Delta E$ , eV |
| +3                     | $T_d$    | 5.11                         |                 |
| +2                     | $T_d$    | 4.63                         |                 |
| +1                     | $C_{2v}$ | 4.76 (1), 4.23 (4), 3.45 (1) | 0               |

|                         | $T_d$    | 4.11                         | 0.045           |
|-------------------------|----------|------------------------------|-----------------|
| 0                       | $T_d$    | 3.87                         | 0               |
|                         | $C_{2v}$ | 4.40 (1), 4.98 (4), 3.46 (1) | 0.016           |
| -1                      | $D_{2d}$ | 3.22 (2), 3.85 (4)           |                 |
| -2                      | $D_2$    | 3.19 (2), 3.62 (4), 3.71 (2) |                 |
| -3                      | $D_{2d}$ | 3.67 (2), 3.21 (4)           |                 |
| PBE, 215-atom supercell |          |                              |                 |
| Charge                  | Symmetry | In-In distances, Å           | $\Delta E$ , eV |
| +3                      | $T_d$    | 5.15                         |                 |
| +2                      | $T_d$    | 4.63                         |                 |
| +1                      | $C_{2v}$ | 4.76 (1), 4.22 (4), 3.41 (1) | 0               |
|                         | $T_d$    | 4.06                         | 0.034           |
| 0                       | $D_{2d}$ | 3.56 (2), 3.90 (4)           | 0               |
|                         | $T_d$    | 3.86                         | 0.058           |
| -1                      | $D_{2d}$ | 3.14 (2), 3.86 (4)           |                 |
| -2                      | $D_{2d}$ | 3.13 (2), 3.75 (4)           |                 |
| -3                      | $D_{2d}$ | 3.68 (2), 3.19 (4)           |                 |

**Table S2.** Symmetry of  $V_{As}$  in InAs and interatomic distances for indium atoms nearest to the vacancy in different charge states. Calculation with PBE functional for supercell sizes of 63 and 215 atoms. If the In-In interatomic distances are different, their number is given in parentheses for each distance. If several different configurations with close total energies are found, the difference in total energies  $\Delta E$  is shown for them relative to the configuration with the minimum energy in a given charge state.

| PBE, 63-atom supercell  |          |                              |                 |
|-------------------------|----------|------------------------------|-----------------|
| Charge                  | Symmetry | In-In distances, Å           | $\Delta E$ , eV |
| +3                      | $T_d$    | 5.28                         |                 |
| +2                      | $T_d$    | 4.80                         | 0               |
|                         | $C_{2v}$ | 5.17 (1), 4.49 (4), 3.27 (1) | 0.271           |
| +1                      | $C_{2v}$ | 5.14 (1), 4.46 (4), 3.28 (1) | 0               |
|                         | $T_d$    | 4.19                         | 0.109           |
| 0                       | $C_{2v}$ | 4.32 (1), 3.98 (4), 3.55 (1) | 0               |
|                         | $T_d$    | 3.93                         | 0.0026          |
| -1                      | $T_d$    | 3.70                         |                 |
| -2                      | $D_{2d}$ | 3.24 (2), 3.70 (4)           |                 |
| -3                      | $D_{2d}$ | 3.70 (2), 3.24 (4)           | 0               |
|                         | $D_{2d}$ | 3.15 (2), 3.58 (4)           | 0.027           |
| PBE, 215-atom supercell |          |                              |                 |
| Charge                  | Symmetry | In-In distances, Å           | $\Delta E$ , eV |
| +3                      | $T_d$    | 5.33                         |                 |
| +2                      | $C_{2v}$ | 5.10 (1), 4.41 (4), 3.27 (1) | 0               |
|                         | $T_d$    | 4.77                         | 0.124           |
| +1                      | $C_{2v}$ | 5.08 (1), 4.41 (4), 3.27 (1) | 0               |
|                         | $T_d$    | 4.10                         | 0.119           |
| 0                       | $C_{2v}$ | 4.65 (1), 4.13 (4), 3.37 (1) | 0               |
|                         | $T_d$    | 3.91                         | 0.013           |
| -1                      | $D_{2d}$ | 3.16 (2), 3.90 (4)           | 0               |
|                         | $T_d$    | 3.70                         | 0.028           |
| -2                      | $D_{2d}$ | 3.14 (2), 3.83 (4)           |                 |
| -3                      | $D_{2d}$ | 3.13 (2), 3.75 (4)           | 0               |
|                         | $D_{2d}$ | 3.71 (2), 3.22 (4)           | 0.058           |

## 2. Diffusion of interstitial P atoms in InP

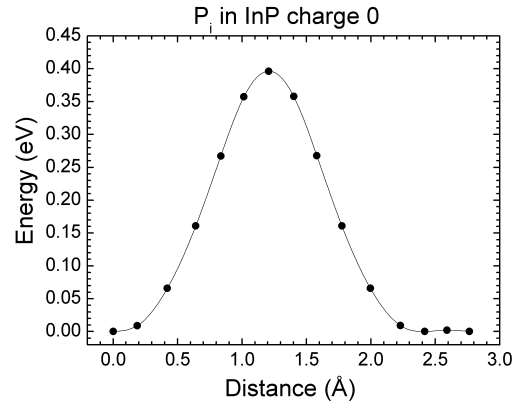

**Figure S5.** Energy profile for movement of a P atom from a neutral split-interstitial with the formation of a split-interstitial near the neighbor site in the [110] direction in the sublattice of P atoms in InP  $(P-P)_i \rightarrow (P-P)_i$ .

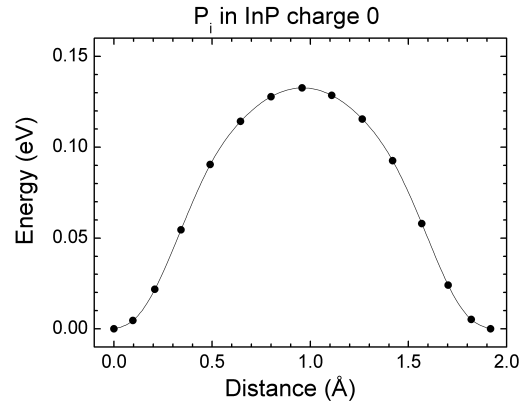

**Figure S6.** Energy profile for 60° rotation of the  $(P-P)_i$  split-interstitial axis in InP in a neutral charge state.

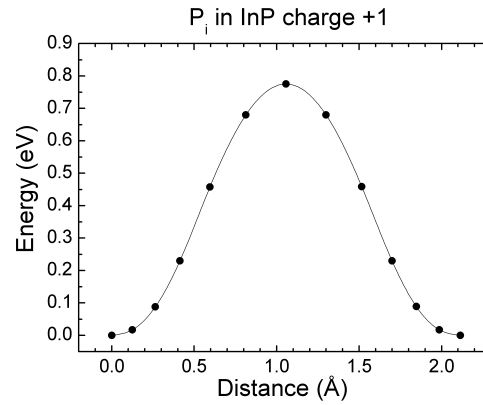

**Figure S7.** Energy profile for transition of an interstitial P atom in InP in the +1 charge state from an In-P split-interstitial site to a neighbor In atom with formation of an In-P split-interstitial with different bond direction  $(In-P)_i \rightarrow (In-P)_i$ .

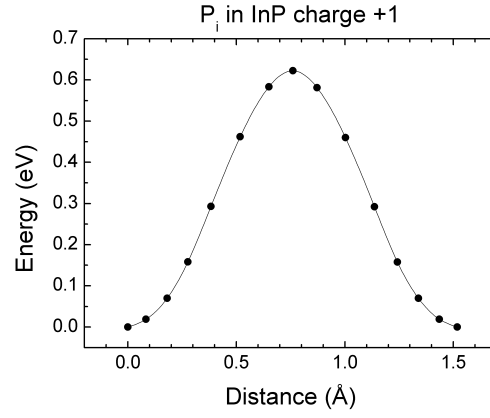

**Figure S8.** Energy profile for rotation of the plane, in which the bonds of the In atom with the interstitial P atom and one of the two P atoms are located, by an angle of  $60^\circ$  for  $P_i$  in InP in the +1 charge state.

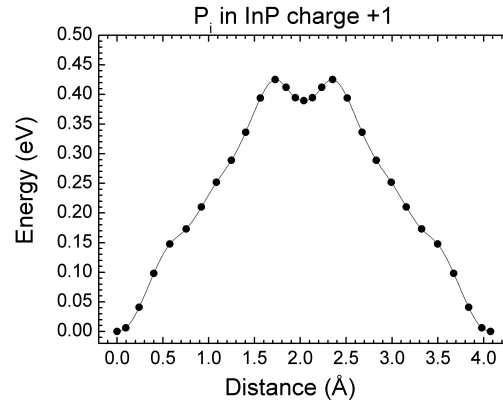

**Figure S9.** Energy profile for transition of an interstitial phosphorous atom in InP in the charge state +1 with a change in the direction of the In-P bond through the metastable split-interstitial state  $(\text{In-P})_i \rightarrow (\text{P-P})_i \rightarrow (\text{In-P})_i$ .

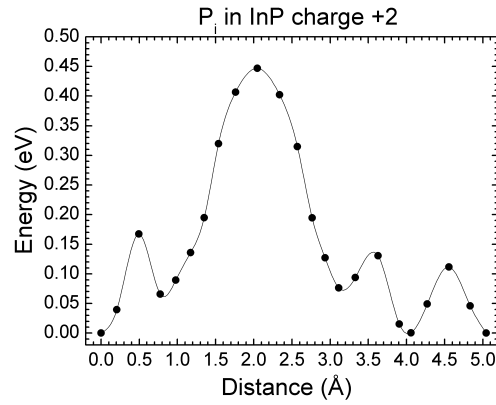

**Figure S10.** Energy profile for migration of an interstitial P atom in InP between the  $C_{3v}$  interstitial positions displaced by one translation vector of the primitive cell for the +2 charge state.

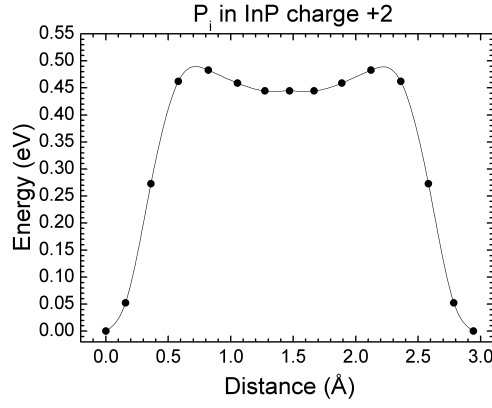

**Figure S11.** Energy profile for transition of an interstitial P atom in InP to a substitution position in the P sublattice with the displacement of the P atom into the interstitial position for the +2 charge state  $P_i + P_P \rightarrow P_P + P_i$ .

### 3. Diffusion of interstitial As atoms in InAs

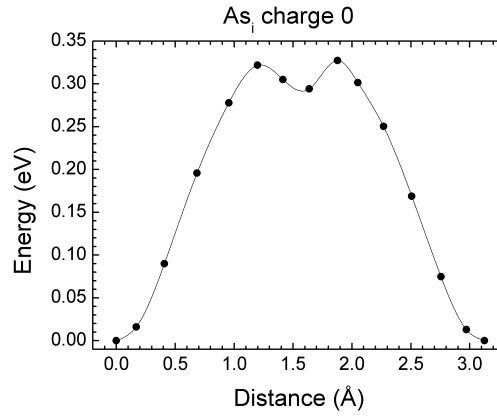

**Figure S12.** Energy profile for movement of a As atom from a neutral split-interstitial with the formation of a split-interstitial near the neighbor site in the [110] direction in the sublattice of As atoms in InAs  $(As-As)_i \rightarrow (As-As)_i$ .

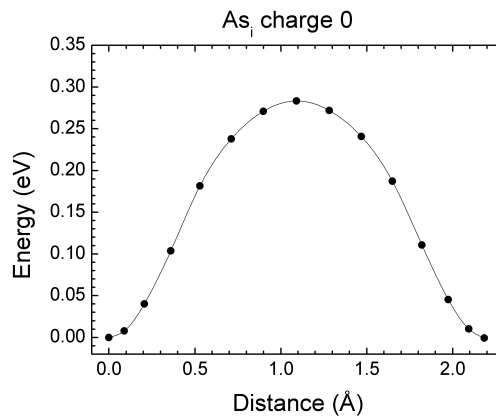

**Figure S13.** Energy profile for 60° rotation of the  $(As-As)_i$  split-interstitial in InAs in a neutral charge state.

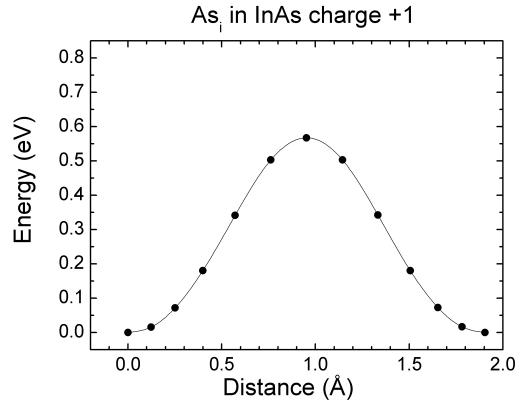

**Figure S14.** Energy profile for transition of an interstitial As atom in InAs in the +1 charge state from an In-As split-interstitial site to a neighbor In atom with formation of an In-As split-interstitial with different bond direction  $(\text{In-As})_i \rightarrow (\text{In-As})_i$ .

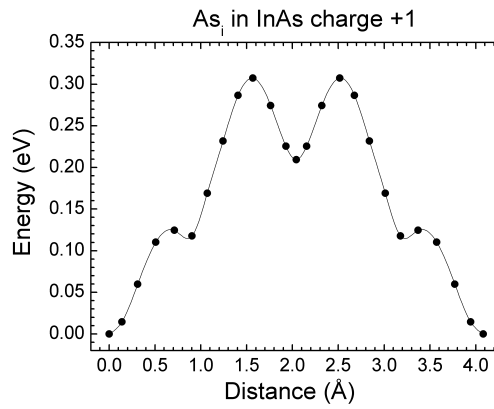

**Figure S15.** Energy profile for transition of an interstitial arsenic atom in InAs in the charge state +1 with a change in the direction of the In-As bond through the metastable split-interstitial state  $(\text{In-As})_i \rightarrow (\text{As-As})_i \rightarrow (\text{In-As})_i$ .

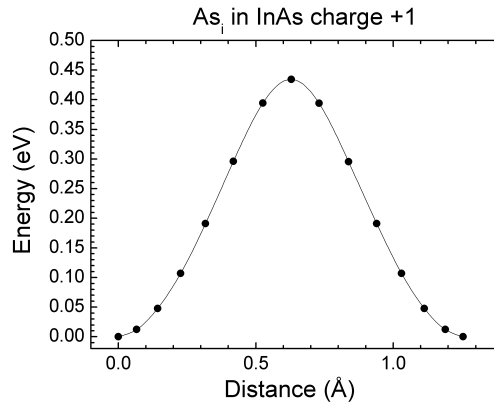

**Figure S16.** Energy profile for rotation of the plane, in which the bonds of the In atom with the interstitial As atom and one of the two As atoms are located, by an angle of  $60^\circ$  for  $\text{As}_i$  in InAs in the +1 charge state.

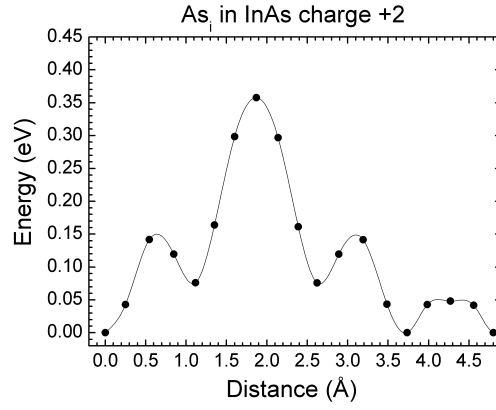

**Figure S17.** Energy profile for migration of an interstitial As atom in InAs between the  $C_{3v}$  interstitial positions displaced by one translation vector of the primitive cell for the +2 charge state.

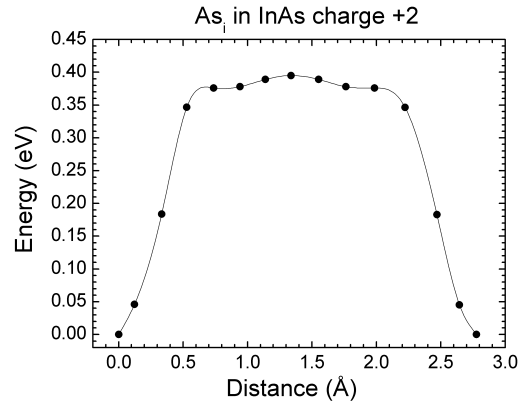

**Figure S18.** Energy profile for transition of an interstitial As atom in InAs to a substitution position in the As sublattice with the displacement of the As atom into the interstitial position for the +2 charge state  $As_i + As_{As} \rightarrow As_{As} + As_i$ .

#### 4. Diffusion of interstitial P atoms in InAs

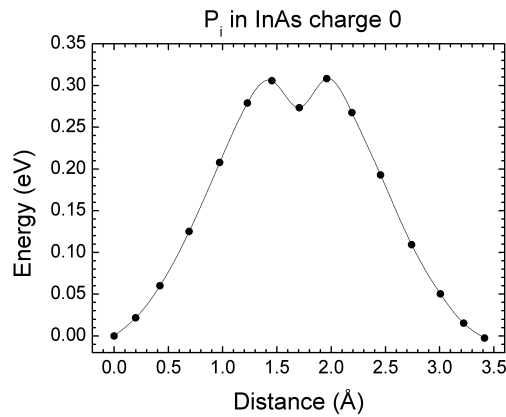

**Figure S19.** Energy profile for movement of a P atom from a neutral split-interstitial with the formation of a split-interstitial near the neighboring site in the [110] direction in the sublattice of As atoms in InAs  $(P-As)_i \rightarrow (P-As)_i$ .



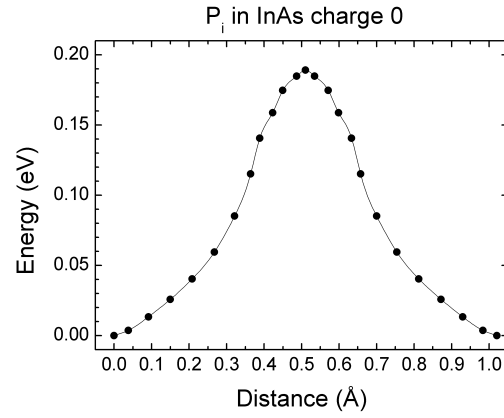

**Figure S20.** Energy profile for 60° rotation of the  $(P-P)_i$  split-interstitial in InAs in a neutral charge state.

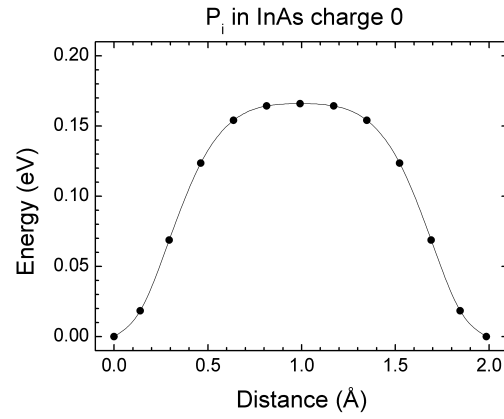

**Figure S21.** Energy profile for 60° rotation (type 2) of the  $P_i$  split-interstitial axis in InAs in a neutral charge state.

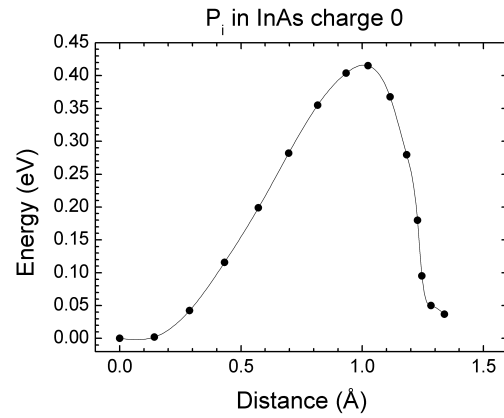

**Figure S22.** Transition of a P atom from a neutral split-interstitial to an As sublattice site with the formation of a split-interstitial consisting of two As atoms  $(P-As)_i \rightarrow P_{As} + (As-As)_i$ .

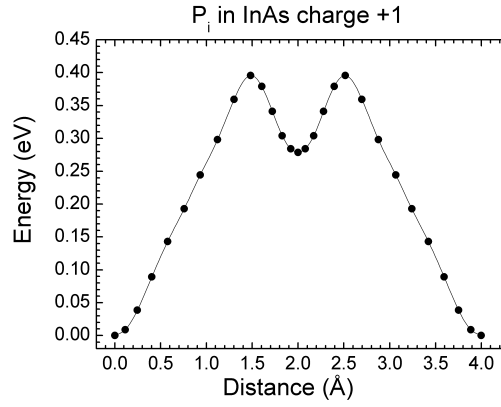

**Figure S23.** Energy profile for transition of an interstitial phosphorous atom in InAs in the charge state +1 with a change in the direction of the In-P bond through the metastable split-interstitial state  $(\text{In-P})_i \rightarrow (\text{P-As})_i \rightarrow (\text{In-P})_i$ .

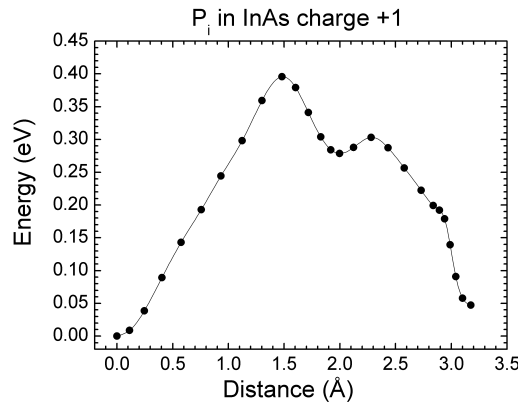

**Figure S24.** Energy profile for transition of an interstitial phosphorous atom in InAs in the charge state +1 in the direction perpendicular to the plane in which the bonds of the In atom with the two nearest As atoms are located through the intermediate metastable split-interstitial state  $(\text{In-P})_i \rightarrow (\text{P-As})_i \rightarrow \text{P}_{\text{As}} + (\text{In-As})_i$ .

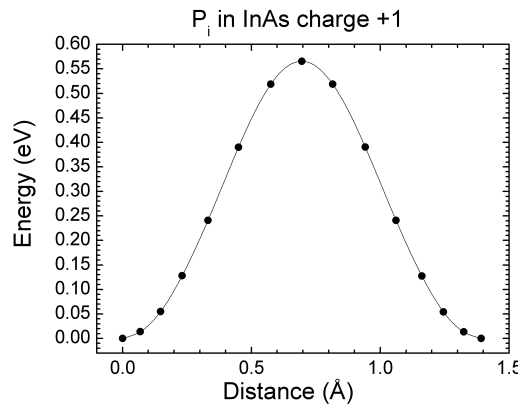

**Figure S25.** Energy profile for rotation of the plane in which the bonds of the In atom with the interstitial P atom and one of the two As atoms are located by an angle of  $60^\circ$  for  $\text{P}_i$  in InAs in the +1 charge state.

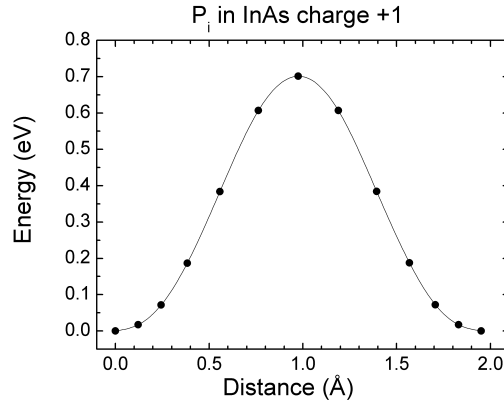

**Figure S26.** Energy profile for transition of an interstitial P atom in InAs in the +1 charge state from an In-P split-interstitial site to a neighbor In atom with formation of an In-P split-interstitial with different bond direction  $(\text{In-P})_i \rightarrow (\text{In-P})_i$ .

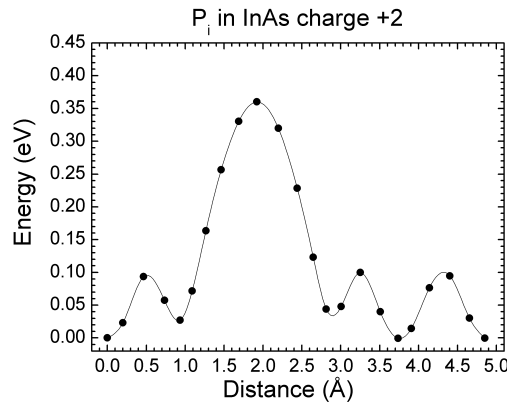

**Figure S27.** Energy profile for migration of an interstitial P atom in InAs between the  $C_{3v}$  interstitial positions displaced by one translation vector of the primitive cell for the +2 charge state.

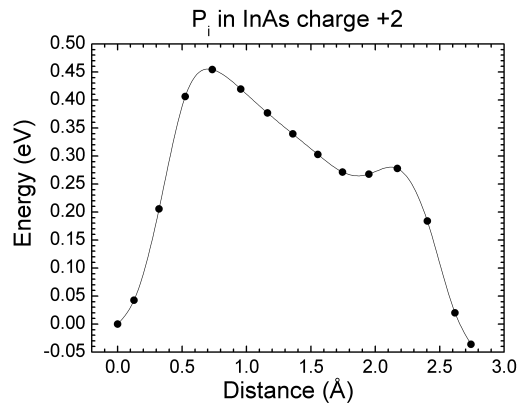

**Figure S28.** Energy profile for transition of an interstitial P atom in InAs to a substitution position in the As sublattice with the displacement of the As atom into the interstitial position for the +2 charge state  $P_i \rightarrow P_{As} + As_i$ .
